# Supplementary material for: Repelling-Attracting Hamiltonian Monte Carlo
Source: arXiv:2403.04607 source file (2024-03-07)
Supplement: Supplementary file 1 [file appendix.tex]

% !TEX root = %WORKSPACE_FOLDER%/plain.tex

\section{Supplementary Results}
\label{sec:supplementary}
