# Supplementary material for: Repelling-Attracting Hamiltonian Monte Carlo
Source: arXiv:2403.04607 source file (2024-03-07)
Supplement: Supplementary file 2 [file exp-appendix.tex]

% !TEX root = %WORKSPACE_FOLDER%/plain.tex
%\section{Results from the experiments}

%\subsection{Dual averaging}
%\label{appendix:exp:da}



%\subsection{Concentric and Nested $\ell_1$ spheres}
%\label{exp:low}


%\subsection{Multimodal Funnel}
%\label{appendix:exp:funnel}




% \begin{table}[!htp]\centering
%     \caption{Results for Anisotropic Gaussian mixtures from Section~\ref{exp:anisotopric}}\label{table:anisotropic}
%     \scriptsize
%     \begin{tabular}{cl | rrrrrr }\toprule
%     {} &\textbf{Method} &${d=2}$ &${d=10}$ &${d=20}$ &${d=50}$ &${d=100}$ \\\midrule
%     \multirow{4}{*}{\bfseries $\mathbf W_2$ metric} &HMC &3.33 &5.55 &8.07 &13.11 &19.56 \\
%     &\haram{} &0.39 &\textbf{0.77} &\textbf{1.35} &\textbf{1.99} &\textbf{3.50} \\
%     &RAM &\textbf{0.26} &5.46 &8.12 &13.50 &20.21 \\
%     &PEHMC &0.71 &3.79 &6.64 &12.41 &18.83 \\ \midrule
%     \multirow{4}{*}{\bfseries ESS} &HMC &\textbf{2890.54} &28.64 &\textbf{367.08} &\textbf{348.31} &\textbf{317.10} \\
%     &\haram{} &1401.32 &\textbf{777.28} &347.73 &10.96 &255.94 \\
%     &RAM &128.16 &46.17 &21.72 &14.51 &18.48 \\
%     &PEHMC &207.60 &219.65 &276.21 &126.45 &107.68 \\ \midrule
%     \multirow{4}{*}{\specialcell{\bfseries Acceptance \\ Rate}} &HMC &71.7\% &82.8\% &59.6\% &91.1\% &97.5\% \\
%     &\haram{} &49.2\% &65.7\% &62.6\% &67.2\% &71.4\% \\
%     &RAM &31.9\% &11.8\% &43.7\% &29.1\% &50.1\% \\
%     &PEHMC &92.0\% &63.6\% &63.5\% &88.5\% &69.2\% \\
%     \bottomrule
%     \end{tabular}
%     \newline
% \end{table}


%\subsection{Anisotropic}
%\label{appendix:exp:anisotropic}

%\begin{figure}[htbp]
%    \centering
%    \begin{subfigure}{\textwidth}
%        \includegraphics[height=0.35\textwidth]{\Root/sims/anisotropic/acf-2d.pdf}
%        \includegraphics[height=0.35\textwidth]{\Root/sims/anisotropic/trace-2d.pdf}
%        \caption{$d=2$}
%    \end{subfigure}

%    \bigskip\bigskip
    
%    \begin{subfigure}{\textwidth}
%        \includegraphics[height=0.35\textwidth]{\Root/sims/anisotropic/acf-10d.pdf}
%        \includegraphics[height=0.35\textwidth]{\Root/sims/anisotropic/trace-10d.pdf}
%        \caption{$d=10$}
%    \end{subfigure}

%    \bigskip\bigskip
    
%    \begin{subfigure}{\textwidth}
%        \includegraphics[height=0.35\textwidth]{\Root/sims/anisotropic/acf-20d.pdf}
%        \includegraphics[height=0.35\textwidth]{\Root/sims/anisotropic/trace-20d.pdf}
%        \caption{$d=100$}
%    \end{subfigure}
%    \caption{ACF plots (left) and trace plots (right) for the anisotropic Gaussian Mixture}
%\end{figure}



%\subsection{Bayesian Neural Network}
%\label{appendix:exp:bnn}
